# Supplementary material for: Emergence of fermionic finite-temperature critical point in a Kondo lattice
Source: arXiv:1604.03737 source file (2016-04-13)
Supplement: Supplementary file 1 [file supplement.pdf]

## SUPPLEMENTARY INFORMATION

# I. RENORMALIZATION GROUP ANALYSIS

## A. Effective Kondo lattice Hamiltonian

To investigate the effective spin interactions between localized spins, we generalize the Kondo lattice Hamiltonian to include the spin-orbit interactions. Upon the application of the the Schrieffer-Wolff transformation[1] on the Anderson lattice Hamiltonian, one obtains the generalized Kondo lattice Hamiltonian[2]. We shall first consider the case of a single localized spin, i.e., a single impurity. The most general Hamiltonian is given by

$$H = \sum_{\mathbf{k}} \begin{pmatrix} \psi_{\mathbf{k}}^{\dagger} & \phi_d^{\dagger} \end{pmatrix} \begin{pmatrix} \xi_{\mathbf{k}} I & M_{\mathbf{k}} \\ M_{\mathbf{k}} & \xi_d I \end{pmatrix} \begin{pmatrix} \psi_{\mathbf{k}} \\ \phi_d \end{pmatrix} + U n_{\uparrow}^d n_{\downarrow}^d, \tag{1}$$

where $\psi_{\mathbf{k}}^{\dagger} = \begin{pmatrix} c_{\mathbf{k}\uparrow}^{\dagger} & c_{\mathbf{k}\downarrow}^{\dagger} \end{pmatrix}$, $\phi_d^{\dagger} = \begin{pmatrix} d_{\uparrow}^{\dagger} & d_{\downarrow}^{\dagger} \end{pmatrix}$, $M_{\mathbf{k}} = v_{\mathbf{k}} I + \vec{v}_{\mathbf{k}} \cdot \vec{\sigma}$, $\xi_{\mathbf{k}} = \varepsilon_k - \mu$, and $\xi_{\mathbf{d}} = \varepsilon_d - \mu$. We first express the Hamiltonian as $H_0 + H_v$ with $H_v$ being the hybridization term and seek a canonical transformation, i.e., the Schrieffer-Wolff transformation[1], $\tilde{H} = e^S H e^{-S} = H + [S,H] + [S,[S,H]] + ...$ such that the $O(H_V)$ term is cancelled. Hence $S$ satisfies $[S, H_0] = -H_v$ and we obtain $\tilde{H} = H_0 + \frac{1}{2}[S, H_v] + ....$

The canonical transformation $S$ can be found and is given by

$$S = \sum_{\mathbf{k}ss'} \left(\frac{1 - n_{-s}^d}{\xi_d - \xi_{\mathbf{k}}} + \frac{n_{-s}^d}{\xi_d + U - \xi_{\mathbf{k}}}\right) M_{\mathbf{k}}^{ss'} d_s^{\dagger} c_{\mathbf{k}s'} - H.C. \tag{2}$$

Substituting back the effective Hamiltonian, $H_{eff} = H_0 + \frac{1}{2}[S, H_v]$, we find that in low energy subspace($n^d = 1$), the extended Kondo interaction terms, $\frac{1}{2}[S, H_v]$, are given by

$$\begin{aligned} \frac{1}{2}[S, H_v] = \sum_{\mathbf{k}\mathbf{k}'} & J'\{(v_{\mathbf{k}} v_{\mathbf{k}'} + \vec{v}_{\mathbf{k}} \cdot \vec{v}_{\mathbf{k}'}) n_{\mathbf{k}\mathbf{k}'} + [v_{\mathbf{k}} \vec{v}_{\mathbf{k}'} + v_{\mathbf{k}'} \vec{v}_{\mathbf{k}} + i(\vec{v}_{\mathbf{k}} \times \vec{v}_{\mathbf{k}'})] \cdot \vec{s}_{\mathbf{k}\mathbf{k}'}\} \\ & + J\{[v_{\mathbf{k}} v_{\mathbf{k}'} (\vec{s}_{\mathbf{k}\mathbf{k}'} \cdot \vec{s}_d)] + [(v_{\mathbf{k}} \vec{v}_{\mathbf{k}'} + v_{\mathbf{k}'} \vec{v}_{\mathbf{k}}) \cdot \vec{s}_d n_{\mathbf{k}\mathbf{k}'} + i(v_{\mathbf{k}} \vec{v}_{\mathbf{k}'} - v_{\mathbf{k}'} \vec{v}_{\mathbf{k}}) \cdot (\vec{s}_{\mathbf{k}\mathbf{k}'} \times \vec{s}_d)] \\ & + [i(\vec{v}_{\mathbf{k}'} \times \vec{v}_{\mathbf{k}}) \cdot \vec{s}_d n_{\mathbf{k}\mathbf{k}'} + (\vec{s}_{\mathbf{k}\mathbf{k}'} \cdot \vec{v}_{\mathbf{k}})(\vec{V}_{\mathbf{k}'} \cdot \vec{s}_d) + (\vec{s}_{\mathbf{k}\mathbf{k}'} \cdot \vec{v}_{\mathbf{k}'})(\vec{v}_{\mathbf{k}} \cdot \vec{s}_d) - (\vec{v}_{\mathbf{k}} \cdot \vec{v}_{\mathbf{k}'})(\vec{s}_{\mathbf{k}\mathbf{k}'} \cdot \vec{s}_d)]\} \end{aligned} \tag{3}$$

where $J' = -\frac{1}{2}(\frac{1}{U+\xi_d-\xi_{\mathbf{k}'}} + \frac{1}{\xi_d-\xi_{\mathbf{k}}})$, $J = \frac{1}{U+\xi_d-\xi_{\mathbf{k}'}} - \frac{1}{\xi_d-\xi_{\mathbf{k}}}$, $\vec{s}_{\mathbf{k}\mathbf{k}'} = \psi_{\mathbf{k}}^{\dagger} \vec{\sigma} \psi_{\mathbf{k}'}$, $n_{\mathbf{k}\mathbf{k}'} = \psi_{\mathbf{k}}^{\dagger} \psi_{\mathbf{k}'}$, and $\vec{s}_d = \phi_d^{\dagger} \frac{\vec{\sigma}}{2} \phi_d$.

In the case we investigated in the paper, we set $v_{\mathbf{k}} = v$, $\vec{v}_{\mathbf{k}} = 2\lambda_{so}\mathbf{k}$, and $\xi_d = -\frac{U}{2}$. By approximating energies near the Fermi surface, the Hamiltonians of spin-interactions are

given by

$$h_1 = J_1 \vec{s}_{\mathbf{k}\mathbf{k}'} \cdot \vec{s}_d,$$
$$h_2 = J_2[(\hat{k} + \hat{k}') \cdot \vec{s}_d n_{\mathbf{k}\mathbf{k}'} - i(\hat{k} - \hat{k}') \cdot (\vec{s}_{\mathbf{k}\mathbf{k}'} \times \vec{s}_d)],$$
$$h_3 = J_3[-i(\hat{k} \times \hat{k}') \cdot \vec{s}_d n_{\mathbf{k}\mathbf{k}'} + (\vec{s}_{\mathbf{k}\mathbf{k}'} \cdot \hat{k})(\hat{k}' \cdot \vec{s}_d) + (\vec{s}_{\mathbf{k}\mathbf{k}'} \cdot \hat{k}')(\hat{k} \cdot \vec{s}_d) - (\hat{k} \cdot \hat{k}')(\vec{s}_{\mathbf{k}\mathbf{k}'} \cdot \vec{s}_d)], \quad (4)$$

where $J_1 = Jv^2$, $J_2 = 2Jv\lambda_{so}k_F$, and $J_3 = 4J\lambda_{so}^2 k_F^2$. Following the poor man's RG analysis[3] and defining dimensionless parameter $g_i = 2\rho J_i$ ($\rho$ is the density of states at the Fermi level), we obtain the flow equation

$$\dot{g_1} = -(g_1^2 + g_2^2),$$
$$\dot{g_2} = -g_2(g_1 + g_3),$$
$$\dot{g_3} = -(g_3^2 + g_2^2). \quad (5)$$

The solution to Eqs.(5) are given by $\frac{g_1 - g_3}{g_2} = const \equiv 2C$, $\dot{u} = -u^2$, and $\dot{w} = -w^2$ with $u = \frac{g_1+g_3}{2} + \sqrt{(\frac{g_1-g_3}{2})^2 + g_2^2}$, $w = \frac{g_1+g_3}{2} - \sqrt{(\frac{g_1-g_3}{2})^2 + g_2^2}$. Since the initial condition (coupling constant at band cut-off $D_0$) satisfied $g_1(D_0)g_3(D_0) = g_2^2(D_0)$, we find that $w_0 = 0$ and $u_0 = 2\rho(J_1 + J_3)$, and three coupling constant flow to infinity at the enhanced Kondo temperature $T_K = D_0 e^{\frac{-1}{2\rho(J_1+J_3)}}$ with solutions of $g_n$ being given by

$$g_1 = \frac{1}{2}(1 + \frac{C}{\sqrt{C^2+1}})\frac{u_0}{1 - u_0 ln(\frac{D_0}{D})},$$
$$g_2 = \frac{1}{2}\frac{1}{\sqrt{C^2+1}}\frac{u_0}{1 - u_0 ln(\frac{D_0}{D})},$$
$$g_3 = \frac{1}{2}(1 - \frac{C}{\sqrt{C^2+1}})\frac{u_0}{1 - u_0 ln(\frac{D_0}{D})}. \quad (6)$$

To exhibit the exact nature of the screening, one takes the continuum limit of the Hamiltonian and and decompose the electron operator in the angular momentum space by setting $C_{\mathbf{k}\sigma} = \sqrt{\frac{V}{(2\pi)^3}} c_{\mathbf{k}\sigma}$, $C_{\mathbf{k}\sigma} = \frac{1}{k}\sum_{lm} \mathrm{Y}_l^m(\hat{k}) C_{lk\sigma}^m$, where $V$ is the volume of the system and $Y_l^m$ are eigenstates of the angular momentum operators. The kinetic energy can be then expressed as $\int d^3k \varepsilon_k C_{\mathbf{k}\sigma}^\dagger C_{\mathbf{k}\sigma} = \int dk \sum_{lm} \varepsilon_k C_{lk\sigma}^{m\dagger} C_{lk\sigma}^m$. The spin-orbital interaction can be expressed as

$$\sum_{\mathbf{k}} \psi_{\mathbf{k}}^\dagger (v + 2\lambda_{so}\vec{\sigma} \cdot \mathbf{k})\phi_d = \sqrt{\frac{V}{(2\pi)^3}} \int d^3k[(v + 2\lambda_{so}k_z)C_{\mathbf{k}\uparrow}^\dagger d_\uparrow + (v - 2\lambda_{so}k_z)C_{\mathbf{k}\downarrow}^\dagger d_\downarrow$$
$$+2\lambda_{so}(k_x - ik_y)C_{\mathbf{k}\uparrow}^\dagger d_\downarrow + 2\lambda_{so}(k_x + ik_y)C_{\mathbf{k}\downarrow}^\dagger d_\uparrow]$$
$$= \sqrt{\frac{V}{2\pi^2}} \int kdk\{[vC_{0k\uparrow}^{0\dagger} + v_{1k}(C_{1k\uparrow}^{0\dagger} + \sqrt{2}C_{1k\downarrow}^{1\dagger})]d_\uparrow + [vC_{0k\downarrow}^{0\dagger} + v_{1k}(-C_{1k\downarrow}^{0\dagger} + \sqrt{2}C_{1k\uparrow}^{-1\dagger})]d_\downarrow, \quad (7)$$

where $v_{1k} = \frac{2}{\sqrt{3}}\lambda_{so}k$. We can further re-express the Hamiltonian in terms of the energy basis by setting $C^m_{lk\sigma} = \sqrt{\frac{d\varepsilon}{dk}}C^m_{l\varepsilon\sigma}$. Hence we obtain $\int dk\varepsilon_k C^{m\dagger}_{lk\sigma}C^m_{lk\sigma} = \int \varepsilon C^{m\dagger}_{l\varepsilon\sigma}C^m_{l\varepsilon\sigma}d\varepsilon$ and

$$\sqrt{\frac{V}{2\pi^2}}\int kdkC^m_{lk\sigma} = \sqrt{\frac{V}{2\pi^2}}\int kd\varepsilon\sqrt{\frac{dk}{d\varepsilon}}C^m_{l\varepsilon\sigma} = \int d\varepsilon\rho(\varepsilon)C^m_{l\varepsilon\sigma}, \tag{8}$$

where $\rho(\varepsilon)$ is the density of states. Finally, the Hamiltonian in energy basis near the Fermi surface becomes

$$H = \int \varepsilon d\varepsilon \sum_{l=0,1}\sum_{m=-l}^{l}\sum_{\sigma} C^{m\dagger}_{l\varepsilon\sigma}C^m_{l\varepsilon\sigma} + \rho\int d\varepsilon\{[vC^{0\dagger}_{0\varepsilon\uparrow} + v_1(C^{0\dagger}_{1\varepsilon\uparrow} - \sqrt{2}C^{1\dagger}_{1\varepsilon\downarrow})]d_\uparrow$$
$$+[vC^{0\dagger}_{0\varepsilon\downarrow} + v_1(-C^{0\dagger}_{1\varepsilon\downarrow} + \sqrt{2}C^{-1\dagger}_{1\varepsilon\uparrow})]d_\downarrow\} + h.c. + \varepsilon_d n_d + Un^d_\uparrow n^d_\downarrow, \tag{9}$$

where $\rho$ is the density of state at the Fermi-level and $v_1 = \frac{2}{\sqrt{3}}\lambda_{so}k_F$.

For a given $z$-component angular momentum, the independent quasi-particles of $c$ electrons can be defined as

$$A^\dagger_{\varepsilon,j_z=\pm\frac{1}{2}} = \frac{1}{\sqrt{v^2+3v_1^2}}[vC^{0\dagger}_{0\varepsilon,\pm\frac{1}{2}} \pm v_1(C^{0\dagger}_{1\varepsilon,\pm\frac{1}{2}} - \sqrt{2}C^{\pm1\dagger}_{1\varepsilon,\mp\frac{1}{2}})],$$
$$B^\dagger_{\varepsilon,j_z=\pm\frac{1}{2}} = \frac{1}{\sqrt{x^2v_1^2+v^2(y^2+z^2)}}[xv_1C^{0\dagger}_{0\varepsilon,\pm\frac{1}{2}} \mp v(yC^{0\dagger}_{1\varepsilon,\pm\frac{1}{2}} + zC^{\pm1\dagger}_{1\varepsilon,\mp\frac{1}{2}})]. \tag{10}$$

Here these quasi-particle operators are properly normalized so that they obey standard anti-commutation relation: $\{A_{\varepsilon,j_z=\pm\frac{1}{2}}, A^\dagger_{\varepsilon,j_z=\pm\frac{1}{2}}\} = 1$ and $\{B_{\varepsilon,j_z=\pm\frac{1}{2}}, B^\dagger_{\varepsilon,j_z=\pm\frac{1}{2}}\} = 1$. Furthermore, $A$ and $B$ anti-commutes as long as $x-y+\sqrt{2}z = 0$ is satisfied. It is clear that $d$ electrons only couple to the quasi-particle operator $A$ with enhanced hybridization strength $\sqrt{v^2+3v_1^2}$ , which corresponds to the enhanced $T_K$. On the other hand, $d$ electrons do not couple with the quasi-particle $B$ operator, which corresponds to the case when $w_0 = 0$. Therefore, even though $T_K$ is enhanced, the spin and orbital degrees of freedom are not completely frozen below $T_K$, which hints that there may exist more structures in the phase space below $T_K$.

To check the exact screening effect, we follow the standard numerical RG (NRG) process[4–6] to compute the capacity ($C_{imp}$) and the spin susceptibility ($\chi_{imp}$) for $c$ and $d$ electrons in 2D systems with total angular momentum being zero. Here the observable $O_{imp}$ is defined as

$$O_{imp} = \frac{Tr(Oe^{-\beta H(J1,R)})}{Tr(e^{-\beta H(J1,R)})} - \frac{Tr(Oe^{-\beta H(J1=0,R=0)})}{Tr(e^{-\beta H(J1=0,R=0)})}, \tag{11}$$

where $R = \frac{2\lambda_{so}}{v}$ is the strength of spin-orbit coupling. The temperature dependence of $C_{imp}$ and $\chi_{imp}$ are shown in Fig. 1. Here $J_1 = -0.1$ is the ordinary Kondo coupling constant

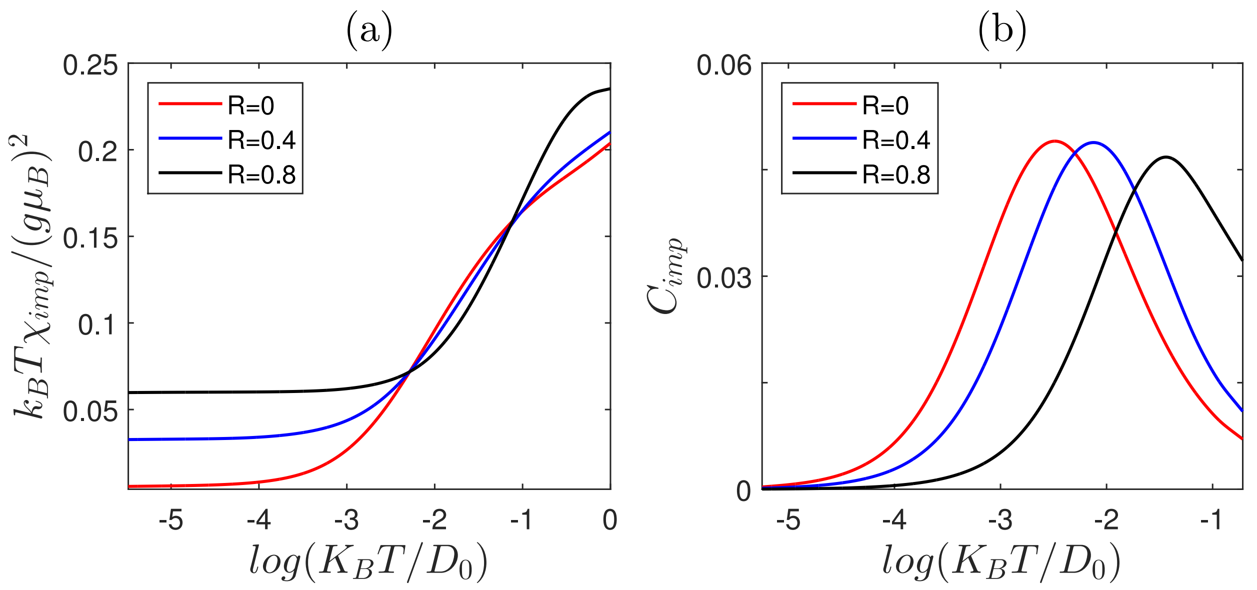


FIG. 1: Temperature dependence of (a) spin susceptibility (b) capacity. Note that both graphs show the enhancement of Kondo temperature. However, at low temperature, the spin susceptibility behavior as $1/T$ with $\chi_{imp}T$ characterizing the magnitude of the residual moments.

defined in Eq(4) and 8000 states were kept in each NRG step. Clearly, the Kondo temperature $T_K$ (characterized by the position of the peak for $C_{imp}$) is enhanced. It is seen that as the strength of spin-orbit interaction increases, the residual moment $T\chi_{imp}$ at zero temperature increases, indicating that localized spins are not screened solely by spins of conduction electrons.

### B. Effective Kondo lattice model

We now extend the renormalization group analysis to the case with many impurities by considering the Kondo lattice model. The Hamiltonian is given by

$$H = \sum_{\mathbf{k}} \begin{pmatrix} \psi^\dagger_{\mathbf{k}} & \phi^\dagger_{\mathbf{k}} \end{pmatrix} \begin{pmatrix} \xi_{\mathbf{k}} I & M_{\mathbf{k}} \\ M_{\mathbf{k}} & \xi_d I \end{pmatrix} \begin{pmatrix} \psi_{\mathbf{k}} \\ \phi_{\mathbf{k}} \end{pmatrix} + U \sum_i n^d_{i\uparrow} n^d_{i\downarrow}, \tag{12}$$

where $\psi^\dagger_{\mathbf{k}} = \begin{pmatrix} c^\dagger_{\mathbf{k}\uparrow} & c^\dagger_{\mathbf{k}\downarrow} \end{pmatrix}$, $\phi^\dagger_{\mathbf{k}} = \begin{pmatrix} d^\dagger_{\mathbf{k}\uparrow} & d^\dagger_{\mathbf{k}\downarrow} \end{pmatrix}$. Here the hybridization term that couples localized spins and conduction electrons is given by $H_v = \sum_{\mathbf{k}} \psi^\dagger_{\mathbf{k}} M_{\mathbf{k}} \phi_{\mathbf{k}} + H.C. = \sum_{\langle ij \rangle} \psi^\dagger_i M_{ij} \phi_j + H.C.$.

To transform the Hamiltonian into an effective Kondo Hamiltonian, consider an operator

$A_j = \sum_{\mathbf{k}ss'}(\frac{1-n^d_{j-s}}{\xi_d-\xi_\mathbf{k}} + \frac{n^d_{j-s}}{\xi_d+U-\xi_\mathbf{k}})B^{ss'}d^\dagger_{js}c_{\mathbf{k}s'} - H.C.$, where $B^{ss'}$ is an arbitrary number. By using Eq.(2), we find that $[A_j, H_0] = -(\sum_{\mathbf{k}ss'} B^{ss'}d^\dagger_{js}c_{\mathbf{k}s'} + H.C.)$. Hence the canonical transformation can be found and is given by

$$S = \sum_{\langle ij\rangle \mathbf{k}ss'}(\frac{1-n^d_{j-s}}{\xi_d-\xi_\mathbf{k}} + \frac{n^d_{j-s}}{\xi_d+U-\xi_\mathbf{k}})\frac{e^{i\mathbf{k}\cdot\mathbf{r}_i}}{\sqrt{N_s}}M^{ss'}_{ij}d^\dagger_{js}c_{\mathbf{k}s'} - H.C.. \tag{13}$$

One can verify that indeed, $[S, H_0] = -(\sum_{\langle ij\rangle\mathbf{k}ss'}\frac{e^{i\mathbf{k}\cdot\mathbf{r}_i}}{\sqrt{N_s}}M^{ss'}_{ij}d^\dagger_{js}c_{\mathbf{k}s'} + H.C.) = -(\sum_{\langle ij\rangle ss'}M^{ss'}_{ij}d^\dagger_{js}c_{is'} + H.C.) = -H_v$ is satisfied. In the case that $\mathbf{k}$ is close to the Fermi surface, we have $|\xi_d| \gg |\xi_\mathbf{k}|$ and $|\xi_d + U| \gg |\xi_\mathbf{k}|$, the transformation is simplified as $S = \sum_{\langle ij\rangle ss'}(\frac{1-n^d_{j-s}}{\xi_d} + \frac{n^d_{j-s}}{\xi_d+U})M^{ss'}_{ij}d^\dagger_{js}c_{is'} - H.C.$.

After performing the Fourier transformation, the extended Kondo interaction terms are given by:

$$\begin{aligned}\frac{1}{2}[S, H_v] = &\sum_{\mathbf{k}\mathbf{k}'} J'\{(v_\mathbf{k}v_{\mathbf{k}'} + \vec{v}_\mathbf{k}\cdot\vec{v}_{\mathbf{k}'})n_{\mathbf{k}\mathbf{k}'} + [v_\mathbf{k}\vec{v}_{\mathbf{k}'} + v_{\mathbf{k}'}\vec{v}_\mathbf{k} + i(\vec{v}_\mathbf{k}\times\vec{v}_{\mathbf{k}'})]\cdot\vec{s}_{\mathbf{k}\mathbf{k}'}\}\\ &+J\{[v_\mathbf{k}v_{\mathbf{k}'}(\vec{s}_{\mathbf{k}\mathbf{k}'}\cdot\vec{s}^d_\mathbf{q})] + [(v_\mathbf{k}\vec{v}_{\mathbf{k}'} + v_{\mathbf{k}'}\vec{v}_\mathbf{k})\cdot\vec{s}^d_\mathbf{q}n_{\mathbf{k}\mathbf{k}'} + i(v_\mathbf{k}\vec{v}_{\mathbf{k}'} - v_{\mathbf{k}'}\vec{v}_\mathbf{k})\cdot(\vec{s}_{\mathbf{k}\mathbf{k}'}\times\vec{s}^d_\mathbf{q})]\\ &+[i(\vec{v}_{\mathbf{k}'}\times\vec{v}_\mathbf{k})\cdot\vec{s}^d_\mathbf{q}n_{\mathbf{k}\mathbf{k}'} + (\vec{s}_{\mathbf{k}\mathbf{k}'}\cdot\vec{v}_\mathbf{k})(\vec{V}_{\mathbf{k}'}\cdot\vec{s}^d_\mathbf{q}) +\\ &(\vec{s}_{\mathbf{k}\mathbf{k}'}\cdot\vec{v}_{\mathbf{k}'})(\vec{v}_\mathbf{k}\cdot\vec{s}^d_\mathbf{q}) - (\vec{v}_\mathbf{k}\cdot\vec{v}_{\mathbf{k}'})(\vec{s}_{\mathbf{k}\mathbf{k}'}\cdot\vec{s}^d_\mathbf{q})]\}\end{aligned} \tag{14}$$

where $J' = -\frac{1}{2}(\frac{1}{U+\xi_d}+\frac{1}{\xi_d})$, $J = \frac{1}{U+\xi_d}-\frac{1}{\xi_d}$, $\vec{s}_{\mathbf{k}\mathbf{k}'} = \psi^\dagger_\mathbf{k}\vec{\sigma}\psi_{\mathbf{k}'}$, $n_{\mathbf{k}\mathbf{k}'} = \psi^\dagger_\mathbf{k}\psi_{\mathbf{k}'}$, $\vec{s}^d_\mathbf{q} = \frac{1}{N_s}\sum_\mathbf{p}\phi^\dagger_{\mathbf{p}+\mathbf{q}}\frac{\vec{\sigma}}{2}\phi_\mathbf{p}$, and $\mathbf{q} = \mathbf{k}' - \mathbf{k}$.

In the lattice model, we set $v_\mathbf{k} = v$, $\vec{v}_\mathbf{k} = 2\lambda_{so}\sin\mathbf{k}$, and $\xi_d = -\frac{U}{2}$. By approximating all energies by their values near the Fermi surface, forms of spin-interactions are given by

$$\begin{aligned}\bar{h}_1 &= \vec{s}_{\mathbf{k}\mathbf{k}'}\cdot\vec{s}^d_\mathbf{q},\\ \bar{h}_2 &= [(\sin\mathbf{k}+\sin\mathbf{k}')\cdot\vec{s}^d_\mathbf{q}n_{\mathbf{k}\mathbf{k}'} - i(\sin\mathbf{k}-\sin\mathbf{k}')\cdot(\vec{s}_{\mathbf{k}\mathbf{k}'}\times\vec{s}^d_\mathbf{q})],\\ \bar{h}_3 &= [-i(\sin\mathbf{k}\times\sin\mathbf{k}')\cdot\vec{s}^d_\mathbf{q}n_{\mathbf{k}\mathbf{k}'} + (\vec{s}_{\mathbf{k}\mathbf{k}'}\cdot\sin\mathbf{k})(\sin\mathbf{k}'\cdot\vec{s}^d_\mathbf{q}) +\\ &\quad(\vec{s}_{\mathbf{k}\mathbf{k}'}\cdot\sin\mathbf{k}')(\sin\mathbf{k}\cdot\vec{s}^d_\mathbf{q}) - (\sin\mathbf{k}\cdot\sin\mathbf{k}')(\vec{s}_{\mathbf{k}\mathbf{k}'}\cdot\vec{s}^d_\mathbf{q})].\end{aligned} \tag{15}$$

Here the complete corresponding Hamiltonian is a summation of $h_1 = J_1\bar{h}_1$, $h_2 = J_2\bar{h}_2$, and $h_3 = J_3\bar{h}_3$ with $J_1 = Jv^2$, $J_2 = 2Jv\lambda_{so}$, and $J_3 = 4J\lambda^2_{so}$.

Performing the poor man's RG analysis[3] to the second order, we obtain contributions

due to the second orders $O(\bar{h}_i\bar{h}_j)$ are given by

$$\begin{aligned}
O(\bar{h}_1^2) &= -2\sum_{\mathbf{q}}\frac{1}{\xi_{\mathbf{q}}}\bar{h}_1,\\
O(\bar{h}_2^2) &= -2\sum_{\mathbf{q}}(\frac{\sin^2\mathbf{q}}{\xi_{\mathbf{q}}}\bar{h}_1+\frac{1}{\xi_{\mathbf{q}}}\bar{h}_3),\\
O(\bar{h}_3^2) &= -2\sum_{\mathbf{q}}\frac{\sin^2\mathbf{q}}{\xi_{\mathbf{q}}}\bar{h}_3,\\
O(\bar{h}_1\bar{h}_2)+O(\bar{h}_2\bar{h}_1) &= -2\sum_{\mathbf{q}}\frac{1}{\xi_{\mathbf{q}}}\bar{h}_2,\\
O(\bar{h}_1\bar{h}_3)+O(\bar{h}_3\bar{h}_1) &= 0,\\
O(\bar{h}_2\bar{h}_3)+O(\bar{h}_3\bar{h}_2) &= -2\sum_{\mathbf{q}}\frac{\sin^2\mathbf{q}}{\xi_{\mathbf{q}}}\bar{h}_2. \qquad (16)
\end{aligned}$$

Here $\sum_{\mathbf{q}}$ denotes the momentum lie in the energy interval $D<\xi_{\mathbf{q}}<D-|\delta D|$. For small $\delta D$, one finds that $\sum_{\mathbf{q}}\frac{1}{\xi_{\mathbf{q}}}=\rho\frac{\delta D}{D}$ and $\sum_{\mathbf{q}}\frac{\sin^2\mathbf{q}}{\xi_{\mathbf{q}}}=\frac{1}{D}\sum_{\mathbf{q}}\sin^2\mathbf{q}\sim C'^2\rho\frac{\delta D}{D}$ with $C'^2$ being a positive number. Clearly, terms listed in Eq.(16) contribute corrections to $J_1\bar{h}_1$, $J_2\bar{h}_2$ and $J_3\bar{h}_3$. Computing coefficients in Eq.(16) and defining $g_1=2\rho J_1$, $g_2=2\rho C' J_2$, and $g_3=2\rho C'^2 J_3$, we obtain the same flow equation as Eq.(5) except that the Kondo temperature is replaced by $T_K=D_0 e^{\frac{-1}{2\rho(J_1+C'^2 J_3)}}$. It is clear that $T_K$ is enhanced in comparison to the Kondo temperature without the spin-orbit coupling, $T_K^0=D_0 e^{\frac{-1}{2\rho J_1}}$.

## II. COMPUTATION OF PHYSICAL RESPONSE FUNCTIONS

The effective Hamiltonian near these Dirac $\mathbf{K}$ points can be expressed as

$$H_{\mathbf{K}}=\begin{pmatrix}(m-\bar{\mu})I & \hbar v_F\sigma\cdot\mathbf{q}\\ \hbar v_F\sigma\cdot\mathbf{q} & -(m+\bar{\mu})I\end{pmatrix}, \qquad (17)$$

where $\mathbf{q}=\mathbf{k}-\mathbf{K}$ is the deviation of the momentum from the Dirac point and $\hbar v_F=2\lambda_{so}a_L$, with $a_L$ is the Lattice constant. In Eq.(17), we have approximated $m_{\mathbf{k}}=\frac{(1+\eta r^2)\varepsilon_{\mathbf{k}}-\varepsilon_d-\lambda}{2}\sim m=\alpha(T-T_D)$ and $\mu_{\mathbf{k}}=\mu-\frac{(1-\eta r^2)\varepsilon_{\mathbf{k}}+\varepsilon_d+\lambda}{2}\sim\bar{\mu}=\bar{\alpha}(T-T_D)$. Note that since $\xi_{\mathbf{k}}=\varepsilon_{\mathbf{k}}-\mu=m_{\mathbf{k}}-\mu_{\mathbf{k}}$, we have $\frac{d\mu}{dT}=\bar{\alpha}-\alpha$. In the following computation, thermodynamics quantities are evaluated by using parameters: $\alpha=0.31k_B$, $\bar{\alpha}=-2.77k_B$, and $\frac{T_D}{\epsilon_c}=0.1$. Here $\epsilon_c=\hbar v_F q_c$. and $n_D$ denote number of the Dirac points.

### A. Self energy

To obtain response functions at finite temperature, in addition to effects due to the Fermi-Dirac distributions, finite lifetime of quasi-particles also contributes[7,8]. For this purpose, we first compute the imaginary part of the self energy for Dirac fermions in the Kondo lattice. Following Ref.[8], the main contribution to the self energy is due to bosons that are not condensed. By expressing the holon operator as $b_i = r + a_i$, the interaction Hamiltonian that goes beyond the mean field theory can be expressed as

$$H_{int} = \sum_{\mathbf{k},\mathbf{q},\sigma,\sigma'} (V_{\mathbf{k}}^{\sigma\sigma'} c^{\dagger}_{\mathbf{k}\sigma} f_{\mathbf{k}+\mathbf{q}\sigma'} a^{\dagger}_{\mathbf{q}} + H.C.). \tag{18}$$

To find the self energy for Dirac fermions in the Kondo lattice, we first write the eigenstate $|psi\rangle$ to the mean field Hamiltonian, Eq.(3), as $|\psi\rangle = (|c\rangle, |f\rangle)$ with $|c\rangle$ and $|f\rangle$ being the corresponding wavefunction for $c$ electrons and spinons with spins being included. The self energy $\Sigma$ can be written as $\Sigma = \Sigma_{ff}|f\rangle\langle f| + \Sigma_{fc}|c\rangle\langle f| + \Sigma_{cf}|f\rangle\langle c| + \Sigma_{cc}|c\rangle\langle c|$. Hence the self energy can be written as

$$\begin{aligned} \Sigma_{\psi\psi} &= \sum_{\sigma,\sigma'} \langle\psi|f_\sigma\rangle\langle f_{\sigma'}|\psi\rangle \Sigma_{ff}^{\sigma\sigma'} + \langle\psi|c_\sigma\rangle\langle f_{\sigma'}|\psi\rangle \Sigma_{fc}^{\sigma\sigma'} \\ &+ \langle\psi|f_\sigma\rangle\langle c_{\sigma'}|\psi\rangle \Sigma_{cf}^{\sigma\sigma'} + \langle\psi|c_\sigma\rangle\langle c_{\sigma'}|\psi\rangle \Sigma_{cc}^{\sigma\sigma'}. \end{aligned} \tag{19}$$

The Green's functions for holons are arranged as a $2 \times 2$ matrix defined by

$$D(k,\tau) = \begin{pmatrix} \langle T_\tau a^{\dagger}_{-\mathbf{k}}(\tau) a_{-\mathbf{k}}(0)\rangle & \langle T_\tau a_{\mathbf{k}}(\tau) a_{-\mathbf{k}}(0)\rangle \\ \langle T_\tau a^{\dagger}_{-\mathbf{k}}(\tau) a^{\dagger}_{\mathbf{k}}(0)\rangle & \langle T_\tau a_{\mathbf{k}}(\tau) a^{\dagger}_{\mathbf{k}}(0)\rangle \end{pmatrix}, \tag{20}$$

where $\tau$ is an imaginary time, $T_\tau$ is the imaginary-time ordering operator, and $\langle\rangle$ denotes an expectation value in the system described by the Hamiltonian. Similarly, the Green's functions for $c$ electrons and spins $f$ are arranged as $2 \times 2$ matrix defined by

$$\begin{aligned} G_c^{\alpha\beta}(k,\tau) &= \langle T_\tau c_{\alpha,\mathbf{k}}(\tau) c^{\dagger}_{\beta,\mathbf{k}}(0)\rangle, \\ G_f^{\alpha\beta}(k,\tau) &= \langle T_\tau f_{\alpha,\mathbf{k}}(\tau) f^{\dagger}_{\beta,\mathbf{k}}(0)\rangle, \\ G_m^{\alpha\beta}(k,\tau) &= \langle T_\tau f_{\alpha,\mathbf{k}}(\tau) c^{\dagger}_{\beta,\mathbf{k}}(0)\rangle. \end{aligned} \tag{21}$$

In the mean field level, one has

$$D = D_0 = \begin{pmatrix} \frac{1}{i\omega - \lambda} & 0 \\ 0 & \frac{1}{-i\omega - \lambda} \end{pmatrix}, \tag{22}$$

where $\omega$ is the Matsubara frequency for bosons. By treating the hybridization as a perturbation, the mean-field Green's functions for $c$ electrons and spins $f$ are found as $G_c^{\alpha\beta} = G_c \delta_{\alpha\beta}$, $G_f^{\alpha\beta} = G_f \delta_{\alpha\beta}$, and $G_m^{\alpha\beta} = (V_{\mathbf{k}}^{\alpha\beta}/V_k)G_m$ with

$$G_c(k, i\omega) = \frac{v_k^2}{i\omega - \epsilon_1(k)} + \frac{u_k^2}{i\omega - \epsilon_2(k)},$$
$$G_f(k, i\omega) = \frac{u_k^2}{i\omega - \epsilon_1(k)} + \frac{v_k^2}{i\omega - \epsilon_2(k)},$$
$$G_m(k, i\omega) = \frac{-V_k r/\Delta_k}{i\omega - \epsilon_1(k)} + \frac{V_k r/\Delta_k}{i\omega - \epsilon_2(k)}. \quad (23)$$

Here $\epsilon_1 = -\Delta_k - \bar{\mu}$, $\epsilon_2 = \Delta_k - \bar{\mu}$, and $\Delta_k = \sqrt{m^2 + \hbar^2 v_F^2 k^2}$. The coherent factors are given by $u_k^2 = (1 + m/\Delta_k)/2$ and $v_k^2 = (1 - m/\Delta_k)/2$.

In the lowest order (one-loop), self energies are given by[8]

$$\Sigma_{ff}(k, i\omega) = \mathbf{I}\frac{-1}{\beta N}\sum_{q,\Omega} r^2 V_{\mathbf{k-q}}^2 G_c(\mathbf{k-q}, i\omega - i\Omega) D_{22}(q, i\Omega),$$
$$\Sigma_{cc}(k, i\omega) = \mathbf{I}\frac{-1}{\beta N}\sum_{q,\Omega} r^2 V_{\mathbf{k}}^2 G_f(\mathbf{k-q}, i\omega - i\Omega) D_{11}(q, i\Omega),$$
$$\Sigma_{fc}(k, i\omega) = \mathbf{V_k}\frac{-1}{\beta N}\sum_{q,\Omega} r^2 V_{\mathbf{k-q}} G_m(\mathbf{k-q}, i\omega - i\Omega) D_{12}(q, i\Omega),$$
$$\Sigma_{cf}(k, i\omega) = \mathbf{V_k}\frac{-1}{\beta N}\sum_{q,\Omega} r^2 V_{\mathbf{k-q}} G_m(\mathbf{k-q}, i\omega - i\Omega) D_{21}(q, i\Omega), \quad (24)$$

where $\beta = k_B T$, $N$ is the number of sites and $\mathbf{I}$ is the unit $2 \times 2$ matrix. By performing analytic continuation $\imath\omega \to \omega + i0^+$ and using the spectral representation, one can convert the frequency summation in Eqs.(24) into

$$\frac{1}{\beta}\sum_{\Omega} G(\mathbf{k-q}, i\omega - i\Omega) D_{ij}(q, i\Omega) =$$
$$\int \frac{d\omega'}{\pi} \sum_{n=1,2} \frac{A_n(\mathbf{k-q})\mathrm{ImD_{ij}}(\mathbf{k-q}, \omega')}{i\omega - \omega' - \epsilon_n(\mathbf{k-q}) + i0^+} \left[n_F(-\epsilon_n(\mathbf{k-q})) + n_B(\omega')\right], \quad (25)$$

where $A_n$ is the corresponding coherent factor to the energy $\epsilon_n$ in $G$, $n_F$ is the Fermi-Dirac distribution function and $n_B$ is the Bose-Einstein distribution function. The imaginary part of the self energy can thus be generally written as

$$\mathrm{Im}\Sigma_{\mathrm{ij}}^{\sigma\sigma'}(\mathrm{k}, \omega) = -\mathrm{s}^{\sigma\sigma'} \sum_{\mathrm{q},\Omega} \mathrm{r}^2 \bar{\mathrm{V}}(\mathbf{k}, \mathbf{q}) \times$$
$$\sum_{n=1,2} A_n(\mathbf{k-q})\mathrm{ImD_{ij}}(\mathbf{k-q}, \omega - \epsilon_{\mathrm{n}}(\mathbf{k-q}) \left[\mathrm{n_F}(-\epsilon_{\mathrm{n}}(\mathbf{k-q})) + \mathrm{n_B}(\omega - \epsilon_{\mathrm{n}}(\mathbf{k-q})\right]. \quad (26)$$

Here $s^{\sigma\sigma'} = \delta_{\sigma,\sigma'}$ if $\Sigma_{ij} = \Sigma_{ff}$ or $\Sigma_{cc}$ while $s^{\sigma\sigma'} = V_{\mathbf{k}}^{\sigma\sigma'}$ when $\Sigma_{ij} = \Sigma_{cf}$ or $\Sigma_{fc}$. The factor hybridization factor $\bar{V}(\mathbf{k},\mathbf{q})$ is equal to $V_{\mathbf{k}}^2$ when $\Sigma_{ij} = \Sigma_{cc}$ and is $V_{\mathbf{k}-\mathbf{q}}^2$ otherwise.

The temperature dependence of $\Sigma_{ij}$ in Eq.(26) is determined by the holon propagator $D_{ij}$ which can be written as

$$D^{-1} = i\omega - \lambda - \Gamma = i\omega - \lambda - \begin{pmatrix} \Gamma^{11} & \Gamma^{12} \\ \Gamma^{21} & \Gamma^{22} \end{pmatrix}, \tag{27}$$

where $\Gamma$ is the self energy for holons. In the lowest one-loop order, we find

$$\begin{aligned} \Gamma^{11}(\mathbf{k}, i\omega) &= \frac{1}{\beta N} \sum_{\mathbf{p},\Omega,\alpha,\beta} G_c^{\alpha\beta}(\mathbf{p}+\mathbf{k}, i\omega + i\Omega) G_f^{\beta\alpha}(\mathbf{p}, i\Omega), \\ \Gamma^{12}(\mathbf{k}, i\omega) &= \Gamma^{21} = \frac{1}{\beta N} \sum_{\mathbf{p},\Omega,\alpha,\beta} G_m^{\alpha\beta}(\mathbf{p}+\mathbf{k}, i\omega + i\Omega) G_m^{\beta\alpha}(\mathbf{p}, i\Omega), \\ \Gamma^{22}(\mathbf{k}, i\omega) &= \frac{1}{\beta N} \sum_{\mathbf{p},\Omega,\alpha,\beta} G_f^{\alpha\beta}(\mathbf{p}+\mathbf{k}, i\omega + i\Omega) G_c^{\beta\alpha}(\mathbf{p}, i\Omega). \end{aligned} \tag{28}$$

Since the transition temperature $T_D$ is much less than the Kondo temperature $T_K$, the low temperature behavior of the self energy $\Sigma_{ij}$ is the main concern. Hence we shall consider the self energy $\Sigma_{ij}$ at finite temperatures in the range: $\omega \sim 0$ and all relevant energies $\epsilon_n \sim 0$. The corresponding range for the holon propagator is $\omega \sim 0$ and $q \sim 0$. Following Ref. [8], in the low temperature regime, one can approximate $n_B(\epsilon) = -\theta(-\epsilon) + \frac{\pi^2}{3} k_B^2 T^2 \delta'(\epsilon)$ and $n_F(\epsilon) = \theta(\epsilon) - \frac{\pi^2}{6} k_B^2 T^2 \delta'(\epsilon)$. For $\eta \ll 1$ and $T < T_D$, since the Fermi level lies on the $\psi_+$ band, the imaginary part of $\psi_+$ is the main contribution to conductivity, this leads to

$$\frac{1}{\tau_+} = \mathrm{Im}\Sigma_{\psi+}(\mathrm{k}, \omega) = \left(\frac{\mathrm{rV_K}}{\epsilon_\mathrm{d} + \lambda - \mu}\right)^2 \frac{\omega^2 + \pi^2(\mathrm{k_B T})^2}{2(\epsilon_\mathrm{d} + \lambda - \mu)} \tag{29}$$

where $\tau_+$ is the lifetime of the Dirac fermions and $V_K$ is the hybridization at the mean field Fermi momentum. Similarly, for $T > T_D$, the Fermi energy lies on the $\psi_-$ band, we obtain the the same formula of $\mathrm{Im}\Sigma_{\psi-}$. Substituting numerical values, we find that $\epsilon_d + \lambda - \mu \sim 0.02t \sim 1 - 10\mathrm{meV}$ and $rV_K \sim 0.002t$. Hence in comparison to conventional heavy Fermion materials, the hybridization $V_K$ is much smaller and hence the broadening effects due to finite temperature is not severe.

### B. Heat capacity

The eigen-energy of Eq.(17) is $E^s_{\mathbf{q}} = -\bar{\mu} + s\Delta_{\mathbf{q}}$, where $\Delta_{\mathbf{q}} = \sqrt{m^2+\epsilon_q^2}$, $s = \pm 1$, $\epsilon_q = \hbar v_F|\mathbf{q}|$. Using $\xi_{\epsilon s}$, the thermal average energy per unit volume is given by

$$U = \frac{2n_D}{L^3}\sum_{\mathbf{q}s}(E^s_{\mathbf{q}}+\mu)f(E^s_{\mathbf{q}}) = \frac{n_D}{\pi^2\hbar^3 v_F^3}\sum_s\int_0^{\epsilon_c}(E^s_\epsilon+\mu)f(E^s_\epsilon)\epsilon^2 d\epsilon. \tag{30}$$

In addition to $U$, the holon propagator also contributes[8]

$$F_B = -\sum_{\mathbf{q}}\int\frac{d\epsilon}{\pi}n_B(\epsilon)\tan^{-1}\frac{\mathrm{Im}\det D^{-1}(q,\epsilon+i0^+)}{\mathrm{Re}\det D^{-1}(q,\epsilon)}. \tag{31}$$

The heat capacity near $T_D$ can be obtained by computing $C = \frac{dU}{dT}|_V - T\frac{d^2F_B}{dT^2}$ in which the first term can be cast in the form

$$\begin{aligned} C(T) &= \frac{n_D}{\pi^2\hbar^3 v_F^3}\sum_s\int_0^{\epsilon_c}[\frac{d(E^s_\epsilon+\mu)}{dT}f(E^s_\epsilon)+(E^s_\epsilon+\mu)\frac{dE^s_\epsilon}{dT}f'(E^s_\epsilon)]\epsilon^2 d\epsilon \\ &= T^3\Phi_c(\alpha,\bar{\alpha},\frac{m}{k_BT},\frac{\epsilon_c}{k_BT},\frac{\bar{\mu}}{k_BT}). \end{aligned} \tag{32}$$

### C. Resistivity

The resistivity is computed by first solving the self-energy due to weak impurities in the self-consistent Born approximation. In this approximation, we have $\Sigma_{im}(\omega) = \frac{n_i u^2}{2L^3}\sum_{\mathbf{q}s}G^s_{\mathbf{q}}(\omega)$ with

$$G^s_{\mathbf{q}}(\omega) = \frac{1}{\hbar\omega - s\Delta_{\mathbf{q}} - \Sigma_{im}(\omega)}. \tag{33}$$

Here $s = \pm$, $\Sigma_{im}$ is the self energy due to impurities, $n_{im}$ is the impurity density, and $u$ is the disorder strength. Substituting the energy dispersion for $\Delta_{\mathbf{q}}$, we obtain the self-consistent equation for $\Sigma$

$$\Sigma_{im}(\omega+i0) = \frac{n_{im}u^2}{2\pi^2}(\hbar\omega+i0-\Sigma_{im})\int_0^{q_c}\frac{q^2dq}{(\hbar\omega+i0-\Sigma_{im})^2-(m^2+\hbar^2v_F^2q^2)}. \tag{34}$$

By defining $\Sigma_{im}(\omega+i0) = \delta(\omega) - i\Gamma_{im}(\omega)$, Eq.(34) can be solved numerically for $\delta(\omega)$ and $\Gamma_{im}(\omega)$. To compute the conductivity, one includes the intrinsic imaginary part of self energy by replacing $\Gamma_{im}(\omega)$ by $\Gamma(\omega) = \Gamma_{im}(\omega) + \mathrm{Im}\Sigma_{\psi\psi}$. We first computes the velocity operator as

$$v_x = \frac{dx}{dt} = \frac{i}{\hbar}[H,x] = v_F\begin{pmatrix}0&0&0&1\\0&0&1&0\\0&1&0&0\\1&0&0&0\end{pmatrix} \tag{35}$$

The resistivity $\rho$ is the inverse of the conductivity $\sigma$, which can be computed by using the Kubo formula

$$\sigma_{xx}(\omega) = \frac{e^2\hbar}{\pi L^3}\sum_{q} Tr(v_x \mathtt{Im}G v_x \mathtt{Im}G). \tag{36}$$

We find

$$\begin{aligned}\sigma_{xx}(\omega) &= \frac{e^2\hbar}{\pi L^3}\sum_{\mathbf{q}} 2v_F^2[\frac{\hbar^2 v_F^2 q_x^2}{E_q^2}(\mathtt{Im}G^+ - \mathtt{Im}G^-)^2 + 2\mathtt{Im}G^+\mathtt{Im}G^-] \\ &= \frac{e^2}{\pi^3\hbar^2 v_F}\int_0^{\epsilon_c} d\epsilon[\frac{\epsilon^4}{3E_\epsilon^2}(\mathtt{Im}G^+ - \mathtt{Im}G^-)^2 + 2\epsilon^2\mathtt{Im}G^+\mathtt{Im}G^-].\end{aligned} \tag{37}$$

In the limit $\epsilon_c \to \infty$, Eq.(37) can be simplified as:

$$\sigma_{xx}(\omega) = \frac{\sqrt{2}e^2}{4\pi^2\hbar^2 v_F}\sqrt{D + \sqrt{D^2 + 4\hbar^2\bar{\omega}^2\Gamma^2}}(\frac{D + \sqrt{D^2 + 4\hbar^2\bar{\omega}^2\Gamma^2}}{6\hbar|\bar{\omega}|\Gamma} + \frac{\Gamma}{\hbar|\bar{\omega}|}), \tag{38}$$

where $\hbar\bar{\omega} \equiv \hbar\omega - \delta$ and $D = \hbar^2\bar{\omega}^2 - (m^2 + \Gamma^2)$.

Eqs.(29) and (34) can be rewritten in a dimensionless form: $\frac{\Sigma(\omega)}{T} = \Sigma_1(\frac{m}{k_BT}, \frac{\hbar\omega}{k_BT}, \frac{\epsilon_c}{k_BT}, \frac{A}{k_BT})$, where $A = \frac{4\pi^2\hbar^3 v_F^3}{n_{im}u^2}$. Hence Eq.(37) can be written as $\sigma_{xx}(\omega) = T\bar{\Phi}_\sigma(\frac{m}{k_BT}, \frac{\hbar\omega}{k_BT}, \frac{\epsilon_c}{k_BT}, \frac{A}{k_BT})$. The exponent $a$ is one and the total conductivity can be expressed as

$$\sigma(T) = \int_{-\infty}^{\infty}\sigma_{xx}(\omega)[-f'(\hbar\omega - \bar{\mu})])d\omega = T\Phi_\sigma(\frac{m}{k_BT}, \frac{\bar{\mu}}{k_BT}, \frac{\epsilon_c}{k_BT}, \frac{A}{k_BT}). \tag{39}$$

The resistivity is then given by $\rho(T) = 1/\sigma(T)$ with the exponent $a = -1$.

### D. Magnetic Susceptibility

The magnetic susceptibility is a sum of three parts: susceptibility of holons, Pauli susceptibility and orbital susceptibility of Dirac fermions. We shall compute them separately and add them together to obtain the final susceptibility.

#### 1. *Susceptibility of holons*

Following Ref.[9], in the presence of a magnetic field $B$, the contribution of holons to the grand potential is

$$\Omega_B = -\sum_{\sigma=\pm 1}\sum_{\mathbf{q}}\int\frac{d\epsilon}{\pi}n_B(\epsilon)\tan^{-1}\frac{\mathrm{Im}\det D^{-1}(q, \epsilon - \mu_B\sigma B + i0^+)}{\mathrm{Re}\det D^{-1}(q, \epsilon - \mu_B\sigma B)}, \tag{40}$$

where $\mu_B$ is the Bohr magneton. The magnetic susceptibility due to holons, $\chi_h$, is then given by $\chi_h = -(\frac{\partial^2\Omega}{\partial B^2})|_{B\to 0}$.

*2. Pauli Susceptibility*

The Pauli susceptibility can be computed by adding a Zeeman term to the Hamiltonian

$$H_{\mathbf{K}}(B) = \begin{pmatrix} (m-\bar{\mu})I + \mu_B B\sigma_z & \hbar v_F \sigma\cdot\mathbf{q} \\ \hbar v_F \sigma\cdot\mathbf{q} & -(m+\bar{\mu}) + \mu_B B\sigma_z I \end{pmatrix} \tag{41}$$

The eigen-energy can be found as $E_{\mathbf{q}}^{ss'} = -\bar{\mu} + s\sqrt{(\Delta_{q_z} + s'\mu_B B)^2 + \hbar^2 v_F^2 (q_x^2 + q_y^2)}$. Here $\Delta_{q_z} = \sqrt{m^2 + \hbar^2 v_F^2 q_z^2}$, $s = \pm 1$, $s' = \pm 1$, and $\mu_B = \frac{e\hbar}{2m_e c}$ is the Bohr magneton. The grand potential per unit volume is given by

$$\Omega = -\frac{n_D}{\beta(2\pi)^3} \sum_{ss',\mathbf{q}} ln(1 + e^{-\beta E_{\mathbf{q}}^{ss'}}). \tag{42}$$

From $\Omega$, the magnetization is computed as

$$M = -\frac{\partial\Omega}{\partial B} = -\frac{n_D\mu_B}{(2\pi)^3} \sum_{ss'} \int f(E_{\mathbf{q}}^{ss'}) \frac{s'(\Delta_{q_z} + s'\mu_B B)}{s\sqrt{(\Delta_{q_z} + s'\mu_B B)^2 + \hbar^2 v_F^2 (q_x^2 + q_y^2)}} d^3q. \tag{43}$$

In the limit $B \to 0$, the dependence on $s'$ drops in eigen-energy. We denote the eigen-enegy by $E_{\mathbf{q}}^s = -\bar{\mu} + s\Delta_{\mathbf{q}}$. After performing the summation over $s'$, the Pauli susceptibility is found as

$$\begin{aligned} \chi_P &= -(\frac{\partial^2\Omega}{\partial B^2})|_{B\to 0} \\ &= -\frac{n_D\mu_B^2}{(2\pi)^3} \sum_s 2\int [f(E_{\mathbf{q}}^s) \frac{\hbar^2 v_F^2 (q_x^2 + q_y^2)}{s\Delta_{\mathbf{q}}^3} + f'(E_{\mathbf{q}}^s) \frac{m^2 + \hbar^2 v_F^2 q_z^2}{\Delta_{\mathbf{q}}^2}] d^3q \\ &= -\frac{n_D\mu_B^2}{3\pi^2} \sum_s \int_0^{q_c} [f(E_q^s) \frac{2\hbar^2 v_F^2 q^2}{s\Delta_q^3} + f'(E_q^s) \frac{3m^2 + \hbar^2 v_F^2 q^2}{\Delta_q^2}] q^2 dq. \end{aligned} \tag{44}$$

Here unlike the usual Pauli-susceptibility, the first term contains all contributions below the Fermi energy and is induced by the spin-orbit interaction. To understand its origin, consider the special case when $m = q_z = 0$, the $4\times 4$ Hamiltonian is reduced to two decoupled $2\times 2$ Hamiltonians with the same form: $H = \hbar v_F q_x\sigma_x + \hbar v_F q_y \sigma_y + \mu_B B\sigma_z$. The eigen-energy is $\pm E$ with corresponding eigen-state $\Psi_\pm^{\mathbf{q}}$, where $E = \sqrt{\mu_B^2 B^2 + \hbar^2 v_F^2 (q_x^2 + q_y^2)}$. We find that the average moment $\langle\vec{\sigma}\rangle$ due to $\Psi_+^{\mathbf{q}}$ is proportional to $(\frac{\hbar v_F q_x}{E}, \frac{\hbar v_F q_y}{E}, \frac{\mu_B B}{E})$, while $\langle\vec{\sigma}\rangle$ due to $\Psi_-^{\mathbf{q}}$ is proportional to $(\frac{-\hbar v_F q_x}{E}, \frac{-\hbar v_F q_y}{E}, \frac{-\mu_B B}{E})$. Therefore, for $E > 0$, all states get negative moment, while for $E < 0$, all states get positive moment. This is reflected in the $s$ dependence in Eq.(43) and it results in the special contribution to susceptibility.

The second terms in Eq.(44) is attributed to the Zeeman splitting at energy $-\tilde{\mu} + \Delta_q$. Note that Eq.(44) implies that the contribution of the second term is positive. At zero temperature and $\bar{\alpha} = 0$, Eq.(44) can be integrated and we find

$$\chi_P = \frac{2n_D\mu_B^2}{3\pi^2\hbar^3 v_F^3}[\frac{3m^2+\epsilon_c^2}{3\sqrt{m^2+\epsilon_c^2}}\epsilon_c - m^2 ln(\frac{\sqrt{m^2+\epsilon_c^2}+\epsilon_c}{|m|})]. \tag{45}$$

*3. Orbital Susceptibility*

If we align the external weak magnetic field along +z-direction, the Hamiltonian can be written as

$$H_{\mathbf{q}}^{\mathbf{K}} = \begin{pmatrix} (m-\bar{\mu})I + \mu_B B\sigma_z & v_F\vec{\sigma}\cdot\vec{\pi} \\ v_F\vec{\sigma}\cdot\vec{\pi} & -(m+\bar{\mu})I + \mu_B B\sigma_z \end{pmatrix}, \tag{46}$$

where $\vec{\pi} = -i\hbar\nabla + \frac{e}{c}\mathbf{A}$ with $\mathbf{A}$ being the vector potential. Following the standard way for treating Landau levels, we express the $\vec{\pi}$ in terms of creation and annihilation operators $a$ and $a^\dagger$: $\pi_+ = \sqrt{\frac{2eB\hbar}{c}}a^\dagger$, $\pi_- = \sqrt{\frac{2eB\hbar}{c}}a$ with $\pi_\pm \equiv \pi_x \pm i\pi_y$. By using $a\varphi_n = \sqrt{n}\varphi_{n-1}$, $a^\dagger\varphi_{n-1} = \sqrt{n}\varphi_n$ with $\varphi_n$ being the eigenstate of $a^\dagger a$, the equation of eigen-energy, $H\psi = E\psi$, can be expressed as

$$\begin{pmatrix} m+\mu_B B-\bar{E} & 0 & v_F\pi_z & v_F\pi_- \\ 0 & m-\mu_B B-\bar{E} & v_F\pi_+ & -v_F\pi_z \\ v_F\pi_z & v_F\pi_- & -m+\mu_B B-\bar{E} & 0 \\ v_F\pi_+ & -v_F\pi_z & 0 & -m-\mu_B B-\bar{E} \end{pmatrix} \begin{pmatrix} c_1|q_z,\varphi_{n-1}\rangle \\ c_2|q_z,\varphi_n\rangle \\ c_3|q_z,\varphi_{n-1}\rangle \\ c_4|q_z,\varphi_n\rangle \end{pmatrix} = 0, \tag{47}$$

where $\bar{E} = E + \bar{\mu}$ and $c_i$ are coefficients to be determined. For $n > 0$, the equation reduces to

$$\begin{pmatrix} m+\mu_B B-\bar{E} & 0 & v_F q_z & \hbar\omega_B\sqrt{n} \\ 0 & m-\mu_B B-\bar{E} & \hbar\omega_B\sqrt{n} & -v_F q_z \\ v_F q_z & \hbar\omega_B\sqrt{n} & -m+\mu_B B-\bar{E} & 0 \\ \hbar\omega_B\sqrt{n} & -v_F q_z & 0 & -m-\mu_B B-\bar{E} \end{pmatrix} \begin{pmatrix} c_1 \\ c_2 \\ c_3 \\ c_4 \end{pmatrix} = 0. \tag{48}$$

The eigen-energy can be found as $E_{n,q_z}^{ss'} = -\bar{\mu} + s\sqrt{(\Delta_{q_z} + s'\mu_B B)^2 + \hbar^2\omega_B^2 n}$, where $\hbar\omega_B = \sqrt{\frac{2eB\hbar v_F^2}{c}}$. Note that for $n = 0$, the eigen-state has a different form with$\begin{pmatrix} 0, & c_2|q_z,\varphi_0\rangle, & 0, & c_4|q_z,\varphi_0\rangle \end{pmatrix}$, which yields the eigen-energy, $E_{0,q_z}^s = -\bar{\mu} - \mu_B B + s\Delta_{q_z}$.

The grand potential per unit volume can be written as

$$\Omega = -\frac{n_D}{\beta L^3}(\frac{eBL^2}{2\pi c\hbar})\sum_{ss',n,q_z} ln(1+e^{-\beta E^{ss'}_{n,q_z}}) = -\frac{n_D eB}{2\beta\pi^2 c\hbar}\int_0^{q_c} dq_z \sum_{ss',n} ln(1+e^{-\beta E^{ss'}_{n,q_z}}). \quad (49)$$

Applying the Euler-Maclaurin formula

$$\sum_{n=1}^{\infty} h(n) = \int_0^{\infty} h(x)dx + \frac{1}{2}(h(\infty)-h(0)) + \frac{1}{12}(h'(\infty)-h'(0)) + ..., \quad (50)$$

we find that the grand potential can be resummed into three terms (the terms $h(\infty)$ and $h'(\infty)$ do not contribute to susceptibility)

$$\begin{aligned}\Omega = -\int_0^{q_c} dq_z\{ & \sum_{ss'} \frac{n_D}{\beta(2\pi)^2\hbar^2 v_F^2}\int_0^{\infty} ln(1+e^{-\beta(s\sqrt{(\Delta_{q_z}+s'\mu_B B)^2+x}-\bar{\mu})})dx \\ + & \sum_{s} \frac{n_D eB}{4\beta\pi^2 c\hbar}[ln(1+e^{-\beta(-\mu_B B+s\Delta_{q_z}-\bar{\mu})}) - ln(1+e^{-\beta(\mu_B B+s\Delta_{q_z}-\bar{\mu})})] \\ + & \sum_{ss'} \frac{n_D e^2 B^2 v_F^2}{12\pi^2 c^2}\frac{f(s\mu_B B+s'\Delta_{q_z}-\bar{\mu})}{s\mu_B B+s'\Delta_{q_z}}\}. \quad (51)\end{aligned}$$

By setting $x = \hbar^2 v_F^2(q_x^2+q_y^2)$, we find that the first term is the same as Eq.(42) and will be included in the Pauli susceptibility. By using the rest two terms, the orbital susceptibility can be computed as

$$\chi_o = -(\frac{\partial^2\Omega}{\partial B^2})|_{B\to 0} = \int_0^{q_c} dq_z \sum_{s'}[\frac{n_D e\mu_B}{\pi^2 c\hbar} f(s'\Delta_{q_z}-\bar{\mu}) + \frac{n_D e^2 v_F^2}{3\pi^2 c^2}\frac{f(s'\Delta_{q_z}-\bar{\mu})}{s'\Delta_{q_z}}]. \quad (52)$$

Here the first term is due to the $n=0$ Landau level with only the spin-down state being occupied. This can be realized by noting that for the non-relativistic Landau level, the energy of the nth level that includes the Zeeman energy is given by $E_n = (n+\frac{1}{2})\hbar\omega_0 \pm \frac{1}{2}\hbar\omega_0$. The moment for each level is proportional to $\mu_B$. Since the degeneracy for each Landau level is proportional to $B$, the total moment is thus proportional to $\mu_B B$, which yields the paramagnetic susceptibility shown in the first term.

The second term is the usual diamagnetic susceptibility. By comparing the coefficients for all contribution, we find that the diamagnetic susceptibility dominates as shown in below: In the SI unit, ratio of strengths for Pauli (spin) susceptibility, paramagnetic susceptibility, and diamagnetic susceptibility is given by $\frac{\mu_B^2 q_c^2}{\hbar v_F}$, $\frac{e\mu_B q_c}{\hbar}$, $\frac{e^2 v_F}{\hbar}$. Clearly, for large $v_F$, the spin susceptibility can be ignored. In this case, the diamagnetic dominates and we find

$$\chi_o = \frac{n_D e^2 v_F}{3\pi^2 c^2\hbar}\sum_s \int_0^{\epsilon_c} d\epsilon \frac{f(s\sqrt{m^2+\epsilon^2}-\bar{\mu})}{s\sqrt{m^2+\epsilon^2}} = \Phi_\chi(\frac{m}{k_B T}, \frac{\bar{\mu}}{k_B T}, \frac{\epsilon_c}{k_B T}). \quad (53)$$

[1] J. R. Schrieffer and P. A. Wolff, Phys. Rev. **149**, 491 (1966).

[2] C. Lacroix and M. Cyrot, Phys. Rev. B **20**, 1969 (1979).

[3] P.W. Anderson, J. Phys. C: Solid St. Phys. **3**, 2436 (1970).

[4] K. G. Wilson Rev. Mod. Phys. **47**, 773 (1975).

[5] H. R. Krishna-murthy, J. W. Wilkins, and K. G. Wilson, K.G., Phys. Rev. B **21**, 1003 (1980).

[6] R. Bulla, T. A. Costi, and T. Pruschke, Rev. Mod. Phys. **80**, 395 (2008).

[7] A. Auerbach and K. Levin, Phys. Rev. Lett. **57**, 877 (1986).

[8] A.J. Millis and P.A. Lee, Phys. Rev. B **35**, 2294 (1987).

[9] N. Read and D. M. Newns, J. Phys. C: Solid State Phys. **16**, 3273 (1983).
